# Supplementary material for: Variational Distillation of Diffusion Policies into Mixture of Experts
Source: arXiv:2406.12538 source file (2024-10-18)
Supplement: Supplementary file 1 [file derivation_depr.tex]

\section{Full Derivation of Learning Objective}
Problem Formulation

\begin{align}
    \theta^* = \arg\min_\theta \int_s\text{KL}(q(x|s;\theta)||D(x|s))ds
\end{align}

Decompose the objective for each component (\todo{cite VIPS}) 
\begin{align*} 
J(\theta) =& -\int_s \int_x q(x|s;\theta)\log\frac{q(x|s;\theta)}{D(x|s)}dxds \\=&\int_s\int_x \sum_o q(o|s)q(x|o,s)[\log D(x|s)- \log q(x|s)]dxds \\=&\int_s \sum_o q(o|s) \int_x q(x|o,s)[\log D(x|s)-\log q(o|s)-\log q(x|o,s) \\&+ \log q(o|x,s)]dxds \\ =&\int_s \sum_o q(o|s)[\int_x q(x|o,s)[\log D(x|s)+\log q(o|x,s))dx+H(q(x|o,s)]] \\ &+ H(q(o|s)) ds 
\end{align*}

Objective for each component
\begin{align}
J_o(\theta)=\mathbb{E}_{s\sim p(s)}[\mathbb{E}_{x\sim q(x|s,o;\theta)}[\log D(x|s)+\log \tilde{q}(o|x,s)]+H[q(x|s,o;\theta)]]
\end{align}

Reparametrization Trick
\begin{align*}
\nabla_\theta J^1_o(\theta) &= \nabla_\theta \mathbb{E}_s \mathbb{E}_{\epsilon \sim N(0, I)}[\log D(h_\theta(\epsilon,s)|s)+\log \tilde{q}(o|h_\theta(\epsilon,s),s)] \\&= \mathbb{E}_s\mathbb{E}_{\epsilon \sim N(0, I)}[\frac{\partial \log D(h_\theta(\epsilon,s)|s)}{\partial h_\theta(\epsilon,s)}\frac{\partial h_\theta(\epsilon,s)}{\partial \theta} \\&\quad\quad\quad +\frac{\partial \log \tilde{q}(o|h_\theta(\epsilon,s),s)}{\partial h_\theta(\epsilon,s)}\frac{\partial h_\theta(\epsilon,s)}{\partial \theta}] \\ &= \mathbb{E}_s\mathbb{E}_{\epsilon \sim N(0,I)}[F_{score}(h_\theta(\epsilon,s),s)\frac{\partial h_\theta(\epsilon)}{\partial \theta}\\&\quad\quad\quad+\frac{\partial \log \tilde{q}(o|h_\theta(\epsilon,s),s)}{\partial h_\theta(\epsilon,s)}\frac{\partial h_\theta(\epsilon,s)}{\partial \theta}]
\end{align*} 

The learning objective for each component:
\begin{align*}
L = -\mathbb{E}
_{s\sim p(s)}[\mathbb{E}_{\epsilon\sim N(0, I)}[F_{score}(h(\epsilon, s),s)h_\theta(\epsilon, s)+\log \tilde{q}(o|h(\epsilon, s),s)]+H[q(x|s,o;\theta)]]
\end{align*}
\subsection{Recursive Gating Update}
Explain why we cannot update the Gating using VIPS: Need log-probability but we only have access to the gradient of log-probability.
Inspired by E-Step from EM algorithm:
\begin{align*}
    p_{\text{target}}(o|s)= \int p(a)p(o|a,s) da= \mathbb{E}_{a\sim p(a)} \left[\frac{p(a|s,o) p_{\theta'}(o|s)}{\sum_o p (a|s,o) p_{\theta'}(o|s)} \right]
\end{align*}
where $\theta'$ is the parameter of the gating network from last step. The gating network $p_\theta(o|s)$ can be updated by minimize the Cross-Entropy loss
\begin{align*}
    J_{\theta} = -\sum_o p_{\text{target}}(o|s)\log p_\theta(o|s)
\end{align*}
