# Supplementary material for: Variational Distillation of Diffusion Policies into Mixture of Experts
Source: arXiv:2406.12538 source file (2024-10-18)
Supplement: Supplementary file 2 [file fullresults.tex]

\newpage
% \begin{table}
%   \caption{Sample table title}
%   \label{sample-table}
%   \centering
%   \begin{tabular}{llllllll}
%     \toprule
%     \multicolumn{2}{c}{Part}                   \\
%     \cmidrule(r){1-2}
%     Name     & Description     & Size ($\mu$m) \\
%     \midrule
%     Franka Kitchen & Input terminal  & $\sim$100     \\
%     Block Push     & Output terminal & $\sim$10      \\
%     Soma     & Cell body       & up to $10^6$  \\
%     \bottomrule
%   \end{tabular}
% \end{table}

\begin{table}[ht]
\centering
\resizebox{\textwidth}{!}{
\begin{tabular}{|c|c|c|c|c|c|c|}
\hline
& \multicolumn{2}{c|}{\textbf{Avoiding}} & \multicolumn{2}{c|}{\textbf{Aligning}} & \multicolumn{2}{c|}{\textbf{Pushing}} \\ \hline
 \textbf{Algorithm} & \textbf{Success Rate} & \textbf{Entropy} & \textbf{Success Rate} & \textbf{Entropy} & \textbf{Success Rate} & \textbf{Entropy} \\ \hline
Disc. Diffusion & $0.94$ & $0.89$ & $0.85$ & $0.62$ & $0.74$ & $0.74$ \\ \hline
DD - 1 step & $0.09$ & $0.25$ & $0.00$ & $0.00$ & $0.00$ & $0.00$ \\ \hline
Cont. Diffusion & $0.96$ & $0.87$ & $0.85$ & $0.67$ & $0.78$ & $0.76$ \\ \hline
CD - 1 step & $0.84$ & $0.76$ & $0.91$ & $0.34$ & $0.70$ & $0.50$ \\ \hline
Consistency Model & $0.82\pm0.05$ & $0.72\pm0.02$ & $0.94\pm0.08$ & $0.32\pm0.14$ & $0.66\pm0.05$ & $0.53\pm0.07$ \\ \hline
EM-GPT & $0.65\pm0.18$ & $0.17\pm0.13$ & $0.00\pm0.00$ & $0.00\pm0.00$ & $0.01\pm0,01$ & $0.00\pm0.00$ \\ \hline
IMC-GPT & $0.75\pm0.08$ & $0.82\pm0.05$ & $0.83\pm0.02$ & $0.27\pm0.09$ & $0.76\pm0.04$ & $0.31\pm0.03$ \\ \hline
% VPD-Gaussian   & X\% & $0.00\pm0.00$ & X\% & $0.00\pm0.00$ & X\% & $0.00\pm0.00$ \\ \hline
\textbf{VPD-DD (Ours)} & $0.92\pm0.02$ & $0.37\pm0.01$ &  $0.70\pm0.05$ & $0.25\pm0.09$ & $0.61\pm0.04$ & $0.66\pm0.05$ \\ \hline
\textbf{VPD-CD (Ours)}  & $0.95\pm0.01$ & $0.72\pm0.12$ & $0.86\pm0.04$ & $0.40\pm0.04$ & $0.85\pm0.02$ & $0.69\pm0.08$ \\ \hline
\hline
& \multicolumn{2}{c|}{\textbf{Stacking 1}} & \multicolumn{2}{c|}{\textbf{Stacking 2}} & \multicolumn{2}{c|}{\textbf{Kitchen}} \\ \hline
\textbf{Algorithm}  & \textbf{Success Rate} & \textbf{Entropy} & \textbf{Success Rate} & \textbf{Entropy} & \textbf{Reward} & \textbf{-} \\ \hline
Disc. Diffusion & $0.89$ & $0.24$ & $0.68$ & $0.12$ & - & - \\ \hline
DD - 1 step & $0.00$ & $0.00$ & $0.00$ & $0.00$ & - & - \\ \hline
Cont. Diffusion & $0.91$ & $0.30$ & $0.70$ & $0.13$ & $4.06$ & - \\ \hline
CD - 1 step & $0.75$ & $0.26$ & $0.53$ & $0.07$ & $4.02$ & - \\ \hline
Consistency Model & $0.68\pm0.06$ & $0.19\pm0.12$ & $0.46\pm0.11$ & $0.03\pm0.05$ & $3.87\pm0.05$\ & - \\ \hline
EM-GPT & $0.58\pm0.06$ & $0.43\pm0.08$ & $0.34\pm0.07$ & $0.27\pm0.05$ & $3.67\pm0.05$ & - \\ \hline
IMC-GPT & $0.54\pm0.05$ & $0.37\pm0.04$ & $0.29\pm0.07$ & $0.17\pm0.07$ & $3.62\pm0.10$ & - \\ \hline
% VPD-Gaussian   & X\% & Y & X\% & Y & X\% & - \\ \hline
\textbf{VPD-DD (Ours)} & X\% & Y & X\% & Y & - & - \\ \hline
\textbf{VPD-CD (Ours)}  & $0.83\pm0.09$ & $0.16\pm0.03$ & $0.57\pm0.06$ & $0.13\pm0.06$ & $3.85\pm0.10$ & - \\ \hline
\hline
& \multicolumn{2}{c|}{\textbf{Block Push}} & \multicolumn{2}{c|}{\textbf{Sorting (Image-based)}} & \multicolumn{2}{c|}{\textbf{Stacking (Image-based)}} \\ \hline
 \textbf{Algorithm} & \textbf{Reward} & \textbf{-} & \textbf{Success Rate} & \textbf{Entropy} & \textbf{Success Rate} & \textbf{Entropy} \\ \hline
Disc. Diffusion & - & - & $0.69$ & $0.16$ & $0.58$ & $0.31$ \\ \hline
DD - 1 step & - & - & $0.20$ & $0.09$ & $0.00$ & $0.00$ \\ \hline
Cont. Diffusion & $0.96$ & - & $0.70$ & $0.19$ & $0.66$ & $0.15$ \\ \hline
CD - 1 step & $0.94$ & - & $0.68$ & $0.14$ & $0.58$ & $0.10$ \\ \hline
Consistency Model & $0.89\pm0.05$ & - & $0.71\pm0.07$ & $0.14\pm0.06$ & $0.625\pm0.008$ & $0.056\pm0.003$ \\ \hline
EM-GPT & $0.88\pm0.04$ & - & $0.73\pm0.03$ & $0.11\pm0.01$ & X\% & Y \\ \hline
IMC-GPT & $0.89\pm0.04$ & - & $0.71\pm0.04$ & $0.14\pm0.03$ & X\% & Y \\ \hline
% VPD-Gaussian   & X\% & - & X\% & Y & X\% & Y \\ \hline
\textbf{VPD-DD (Ours)} & - & - & X\% & Y & $0.78\pm0.05$ & $0.08\pm0.02$ \\ \hline
\textbf{VPD-CD (Ours)}  & $0.91\pm0.03$ & - & $0.75\pm0.04$ & $0.17\pm0.02$ & $0.58\pm0.05$ & $0.12\pm0.02$ \\ \hline
\end{tabular}
}
\vspace{10pt}
\caption{Results of Different Algorithms on Various Datasets}
\end{table}
